# Supplementary material for: Chiral magnetoresistance in Pt/Co/Pt zigzag wires
Source: arXiv:1703.07590 source file (2017-03-22)
Supplement: Supplementary file 1 [file SupplementaryMaterial_FinalVersion.pdf]

# Supplementary Material

## Chiral magnetoresistance in Pt/Co/Pt zigzag wires

Yuxiang Yin[1], Dong-Soo Han[1], June-Seo Kim[1], Reinoud Lavrijsen[1], Kyung-Jin Lee[2, 3], Seo-Won Lee[2], Kyoung-Whan Kim[4, 5], Hyun-Woo Lee[6], Henk J. M. Swagten[1], and Bert Koopmans[1]

[1]*Department of Applied Physics, Center for NanoMaterials, Eindhoven University of Technology, PO Box 513, 5600 MB Eindhoven, the Netherlands*

[2] *Department of Materials Science and Engineering, Korea University, Seoul 02841, Korea*

[3] *KU-KIST Graduate School of Converging Science and Technology, Korea University, Seoul 02841, Korea*

[4]*Center for Nanoscale Science and Technology, National Institute of Standards and Technology, Gaithersburg, Maryland 20899, USA*

[5] *Maryland NanoCenter, University of Maryland, College Park, Maryland 20742, USA*

[6] *PCTP and Department of Physics, Pohang University of Science and Technology, Pohang 37673, Korea*

## 1. Derivation of chiral DW resistance

In a magnetic system, the intrinsic DW resistance originates from the mistracking of the conduction electrons with the magnetization profile in a DW, according to the Levy-Zhang theory [S1]. The intrinsic resistance $R_{\text{intrinsic}}$ due to an inhomogeneous magnetic structure is given by

$$R_{\text{intrinsic}} = \int dx C \left(\frac{\partial \mathbf{m}}{\partial x}\right)^2, \tag{S1}$$

where $C$ is a proportionality constant, $\mathbf{m}$ the magnetization and $x$ the position along the DW. We adopt the Rashba Hamiltonian of conduction electrons to describe the chiral spin precession. According to a recent study of the Rashba Hamiltonian [S2], the chiral spin precession makes various spin-related properties chiral. Interestingly, diverse chiral properties can be obtained by replacing conventional derivative $\partial_x \mathbf{m}$ in non-chiral spin properties with the so-called chiral derivative

$$\partial_x \mathbf{m} \to \tilde{\partial}_x \mathbf{m} \quad \text{where} \quad \tilde{\partial}_x \mathbf{m} = \partial_x \mathbf{m} + k_{\text{R}}(\hat{\mathbf{z}} \times \hat{\mathbf{x}}) \times \mathbf{m}, \tag{S2}$$

where z is the interface normal. We apply this replacement to the non-chiral DW resistance in order to obtain a testable prediction of chiral DW resistance

$$R_{\text{intrinsic}} = \int dx C \left(\tilde{\partial}_x \mathbf{m}\right)^2 = \int dx C \left[\left(\frac{\partial \mathbf{m}}{\partial x}\right)^2 + 2k_{\text{R}} \hat{\mathbf{y}} \cdot \left(\mathbf{m} \times \frac{\partial \mathbf{m}}{\partial x}\right)\right] + O(k_{\text{R}}^2), \tag{S3}$$

$k_{\text{R}} = \frac{2\alpha_{\text{R}} m_{\text{e}}}{\hbar^2}$, where $\alpha_{\text{R}}$ is the Rashba coefficient, $m_{\text{e}}$ the mass of electron, and $\hbar$ the reduced Planck constant. Here, we approximate the DW profile as the Walker profile [S3]

$$\mathbf{m} = \left(\text{sech}\left[\frac{(x-X)}{\lambda}\right] \sin\phi, \text{sech}\left[\frac{(x-X)}{\lambda}\right] \cos\phi, \tanh\left[\frac{(x-X)}{\lambda}\right]\right),$$

(S4)

where $\lambda$ represent the DW width, and $\phi$ stands for the DW in-plane angle in between Néel state ($\phi = \frac{\pi}{2}$) and Bloch state ($\phi = 0$). Then the final form of DW resistance can be expressed as

$$R_{\mathrm{intrinsic}} = 2C\left(\frac{1}{\lambda} \pm k_{\mathrm{R}}\pi\sin\phi\right). \tag{S5}$$

The first term on the right side of Eq. (S5) represents a conventional DW resistance from Levy-Zhang's theory [S1], while the second one is a newly derived term induced by the Rashba effect. Interestingly, the new term shows a $\sin\phi$ dependence, indicating that the resistance depends on the chirality of the DW (from now on, we refer to this as chiral resistance), the $+$ ($-$) sign corresponds to an up-down (down-up) DW. Note that the Rashba effect prefers a specific chirality regardless of the current direction (or a sign of wave vector $k$), which allows us to perform an electrical measurement using an AC current source.

Apart from these two contributions from Eq. (S5), a third contribution to the resistance originates from the well-known anisotropic magnetic resistance (AMR) [S4], which also depends on the DW angle. We can therefore write the total DW resistance as

$$R_{\mathrm{DW}\pm} = R_{\mathrm{AMR}} + R_{\mathrm{LZ}} + R_{\mathrm{chiral}} = \Delta R_{\mathrm{AMR}}\sin^2\phi + 2C\left(\frac{1}{\lambda} \pm k_{\mathrm{R}}\pi\sin\phi\right), \tag{S6}$$

## 2. DW width variation

By applying the Walker ansatz, one can derive the DW energy as a function of DW width $\lambda$ and DW angle $\phi$ [S5]

$$E_{\pm} = \frac{2A}{\lambda} + (\mu_0 H_{\mathrm{k}} + \mu_0 H_{\mathrm{d}}\sin^2\phi)M_{\mathrm{S}}\lambda - (\pm D + \mu_0 H_x M_{\mathrm{S}}\lambda)\pi\sin\phi, \tag{S7}$$

where $\pm$ sign corresponds to up-down and down-up DWs, respectively, $H_{\mathrm{k}}$ is the perpendicular (easy axis) anisotropy, $H_{\mathrm{d}}$ is the anisotropic demagnetizing field, $D$ is the DMI parameter, and $H_x$ is an external in-plane field along $x$ direction.

The energy minimizing configuration can be found by

$$\frac{\partial E_{\pm}}{\partial(\sin\phi)} = 2\mu_0 H_{\mathrm{d}} M_{\mathrm{S}}\lambda\sin\phi - \pi(\pm D + \mu_0 H_x M_{\mathrm{S}}\lambda) = 0, \tag{S8}$$

which gives

$$\sin\phi = \frac{\pi}{2}\frac{\pm D + \mu_0 H_x M_{\mathrm{S}}\lambda}{\mu_0 H_{\mathrm{d}} M_{\mathrm{S}}\lambda}, \tag{S9}$$

which is the Eq. (2) in the main text.

Note also that the DW width can vary due to the applied field. Therefore Eq. (S9) does not show explicitly the dependence of $\sin\phi$ as a function of $H_x$. We below figure out the DW width as a function of $H_x$. To see this, we take the derivative with respect to $\lambda$.

$$\frac{\partial E_{\pm}}{\partial \lambda} = -\frac{2A}{\lambda^2} + (\mu_0 H_{\mathrm{k}} + \mu_0 H_{\mathrm{d}} \sin^2\phi) M_{\mathrm{S}} - \pi \mu_0 H_x M_{\mathrm{S}} \lambda \sin\phi = 0, \tag{S10}$$

which gives

$$\lambda^2 = \frac{2A}{(\mu_0 H_{\mathrm{k}} + \mu_0 H_{\mathrm{d}} \sin^2\phi) M_{\mathrm{S}} - \pi \mu_0 H_x M_{\mathrm{S}} \lambda \sin\phi}. \tag{S11}$$

Combination of Eqs. (S9) and (S11) gives the equilibrium configuration. After some algebra,

$$\lambda^2 = \frac{8A\mu_0 H_{\mathrm{d}} M_{\mathrm{S}} - \pi^2 D^2}{4\mu_0^2 H_{\mathrm{d}} H_{\mathrm{k}} M_{\mathrm{S}}^2 - \pi^2 \mu_0^2 H_x^2 M_{\mathrm{S}}^2} = \frac{\lambda_0^2}{1 - (\pi^2 H_x^2 / 4 H_{\mathrm{d}} H_{\mathrm{k}})}, \tag{S12}$$

where $\lambda_0$ is the DW width in the absence of the in-plane field.

Now, let us get back to the equilibrium angle $\phi$. Putting Eq. (S12) into Eq. (S9), the equilibrium angle $\phi$ is given by

$$\sin\phi = \frac{\pi}{2} \frac{\pm D^* + \mu_0 H_x M_{\mathrm{S}} \lambda_0}{\mu_0 H_{\mathrm{d}} M_{\mathrm{S}} \lambda_0}, \tag{S13}$$

where the "renormalized" DMI parameter $D^*$ is given by

$$D^* = D \sqrt{1 - \frac{\pi^2 H_x^2}{4 H_{\mathrm{d}} H_{\mathrm{k}}}}. \tag{S14}$$

Eq. (S14) now gives a correct $H_x$ dependence of $\sin\phi$. By using the parameters in our main text, $\mu_0 H_x = 30$ mT, $\mu_0 H_{\mathrm{d}} = 30$ mT, and $\mu_0 H_{\mathrm{k}} = 650$ mT one can get the $D^* \approx 0.95\, D$, which is small so that the effect of DW width variation can be ignored.

## 3. Quantification of the DMI by the field shift

From Eq. (1) in the main text, the minimum point is given by $\partial R_{\mathrm{DW}} / \partial(\sin\phi) = 0$, after some algebra,

$$\sin\phi = \mp \frac{R_{\mathrm{chiral}}}{2\Delta R_{\mathrm{AMR}}}, \tag{S15}$$

at $H_x = H_{\mathrm{min}}$. By equating this with Eq. (2), we obtain

$$H_{\min} = \mp H_{\mathrm{DMI}} \mp \frac{H_{\mathrm{d}} R_{\mathrm{chiral}}}{\pi \Delta R_{\mathrm{AMR}}}, \tag{S16}$$

which allows to determine $D$ independently of $k_{\mathrm{R}}$ and $\Delta R_{\mathrm{AMR}}$.

## 4. The real-time DW resistance measurement

A wide-field Kerr microscope is used for real-time imaging of the magnetic configuration. When a magnetic field is applied, the Ga-irradiated regions switch first and a pair of DWs get pinned at the boundary. Since the nucleation fields of each irradiation region are not identical, the DWs appears subsequently. Each step observed corresponds to an event that several DWs appears, as shown in Fig. S1. The measurement scheme that combines the electric and the optical methods allows for exclusion of artifacts caused by magnetoresistive effects, such as the tilting of DW profile.

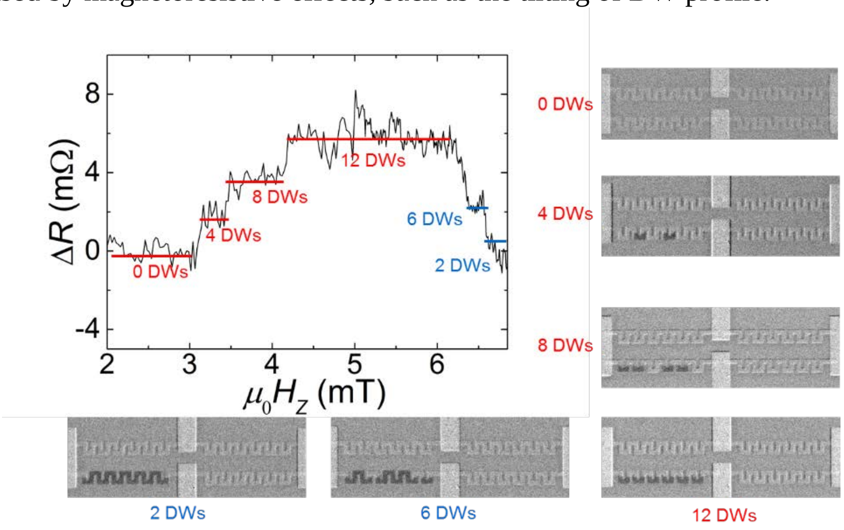


FIG. S1. A measurement of the change in resistance due to the appearance of DWs in a Pt/Co/Pt zigzag wire. The stepwise increase of the resistance is visualized by solid red (solid blue) lines for appearing (disappearing) DWs. The corresponding Kerr microscope images are also shown.

## 5. Determination of the anisotropic magnetoresistance

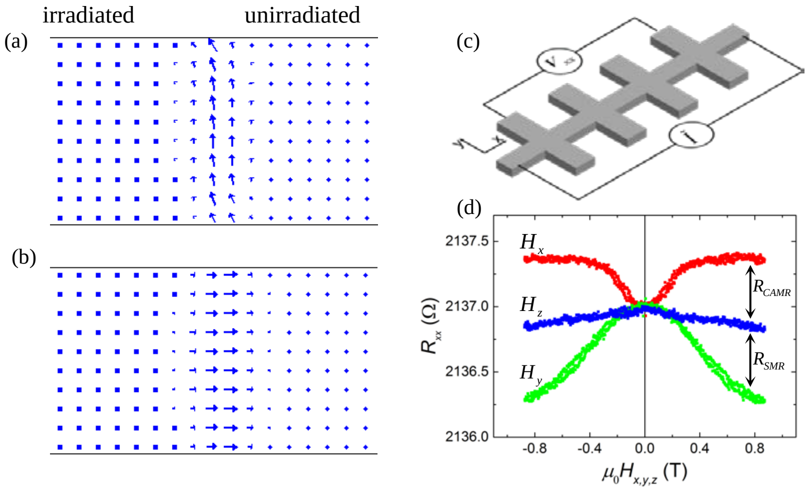


FIG. S2. (a)(b) The viewgraphs show OOMMF simulations of the spin profile of a Bloch-type DW (a) and a Néel-type DW (b). The left part parameterizes a low PMA due to the irradiation. (c) Schematics for the measurements of AMR in a magnetic wire. (d) Longitudinal resistance $R_{\mathrm{xx}}$ as a function of the applied field $\mu_0 H$ for three directions of the field for a Pt(4 nm)/Co(0.5 nm)/Pt(2 nm) wire at room temperature. The differences in resistance $R_{\mathrm{CAMR}}$ and $R_{\mathrm{SMR}}$ represent the conventional AMR and SMR, respectively.

To quantitatively determine the contributions from the AMR, we conducted a micromagnetic simulation using the OOMMF code [S6]. For this simulation, we used the anisotropy constant $K_1 =$

$1.5\ \mathrm{MJ\cdot m^{-3}}$, the DMI energy density $D_1 = 0.05\ \mathrm{mJ\cdot m^{-2}}$ for the unirradiated region and $K_2 = 1.375\ \mathrm{MJ\cdot m^{-3}}$,$D_2 = 0.035\ \mathrm{mJ\cdot m^{-2}}$ for the irradiated region. The saturation magnetization $M_S = 1070\ \mathrm{kA/m}$ was determined with VSM-SQUID magnetometry, the bulk exchange constant $A = 16\times 10^{-12}\ \mathrm{J/m}$ and a high damping rate of 0.5 to allow for a quick relaxation. The simulation cell size was set to 4 nm. From this simulation we calculate the increase of resistance during the transformation to a Néel wall taking into account the AMR effect. For that, the resistance of each cell was calculated by $R_{\mathrm{AMR}} = \Delta R\cos^2\theta$ with $\theta$ being the angle between the magnetization and the current direction. The angle $\theta$ for each cell can be extracted from the DW profile in the simulation, shown in Fig. S2(a)(b). The value for $\Delta R$ is experimentally determined using magnetoresistance (MR) measurements on a Hall bar structure as depicted in Fig. S2(c). The MR of the films has been studied by sweeping magnetic fields in $x, y, z$ directions and we refer to MR of each direction as $R_x, R_y$ and $R_z$. In Fig. S2(d) the MR results for a Pt(4 nm)/Co(0.5 nm)/Pt(2 nm) sample are shown. As can be seen from this figure, two kinds of MR contribute to $\Delta R$, which are the conventional AMR ($R_{\mathrm{CAMR}}$) and newly found spin Hall MR ($R_{\mathrm{SMR}}$) [S7]. In order to quantify these two values accurately, we employed a method from Ref. [S8] and the resultant resistivity is found to be $\Delta\rho = \rho_{\mathrm{CAMR}} + \rho_{\mathrm{SMR}} = 4.3\times 10^{-8}\ \mathrm{m}\cdot\Omega$. By combining the simulation and experiment, one can calculate the AMR for each cell and therefore for the DW, i.e., $\Delta R_{\mathrm{AMR}} = 86\ \mathrm{m}\cdot\Omega$, which is comparable to the values extracted from the DW resistance measurement , as listed in Table S1.

## 6. Straight Pt/Co/Pt wire: fitting the experimental data

In the main text, as shown in Fig. 4(a), DW resistance with different chiralities in the zigzag wire is fitted by the model

$$R_{\mathrm{DW}\pm} = \Delta R_{\mathrm{AMR}}\sin^2\phi + 2\rho_{\mathrm{DW}}\left(\frac{1}{\lambda} \pm k_{\mathrm{R}}\pi\sin\phi\right). \tag{S17}$$

In comparison, due to the fact that DWs with different chiralities are both present in the straight wires, the DW resistance of the straight wires is fitted by $R_{\mathrm{DW}+} + R_{\mathrm{DW}-}$, as shown in Fig. 4(b) and the fitting parameters are listed in Table S1. In order to confirm that chiral DW resistance is indeed averaged out in the straight wires, here we naively perform a similar fit as to the zigzag wires, i.e., by $R_{\mathrm{DW}+}$ instead of by $R_{\mathrm{DW}+} + R_{\mathrm{DW}-}$. Fitting results are shown in Fig. S4 and the parameters obtained are listed in Table S1 (last two rows). By looking at the fitting parameters in Table S1, one can easily tell that the $D$ and $k_{\mathrm{R}}$ of the straight wires are significantly smaller than that of the zigzag wires, demonstrating that the field shift due to the DMI ($D$) and the chiral DW resistance due to the Rashba effect ($k_{\mathrm{R}}$) are cancelled out in the straight wires.

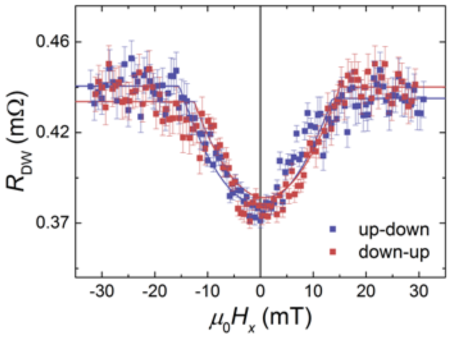


FIG. S3. The measured single DW resistance as a function of in-plane field on a straight wire. The blue and red squares represent the magnetic switching with different polarities (up-down and down-up, respectively). The blue and red solid lines are fits to the data based on the theoretical model.

| | | $D\,(\mathrm{mJ\cdot m^{-2}})$ | $k_\mathrm{R}$ $(\times 10^6\mathrm{m^{-1}})$ | $\mu_0 H_\mathrm{d}$ (mT) | $\Delta R_\mathrm{AMR}$ (m$\Omega$) | $\rho_\mathrm{DW}(\times 10^{-9}\ \mathrm{m\cdot\Omega})$ |
|---|---|---|---|---|---|---|
| Zigzag #1 Fig. 4(a) | Up-down | $-0.049 \pm 0.006$ | $-1.39 \pm 0.09$ | $35.4 \pm 1.5$ | $52 \pm 3$ | $1.41 \pm 0.05$ |
| | Down-up | $-0.048 \pm 0.006$ | $-1.47 \pm 0.10$ | $34.4 \pm 1.4$ | $48 \pm 2$ | $1.41 \pm 0.05$ |
| Zigzag #2 Fig. S4 | Up-down | $-0.047 \pm 0.006$ | $-1.24 \pm 0.07$ | $22.4 \pm 1.1$ | $38 \pm 2$ | $1.16 \pm 0.05$ |
| | Down-up | $-0.046 \pm 0.006$ | $-1.05 \pm 0.06$ | $26.6 \pm 1.3$ | $35 \pm 2$ | $1.17 \pm 0.05$ |
| Straight Fig. 4(b) | Up-down | $-0.035 \pm 0.006$ | – | $16.0 \pm 0.6$ | $63 \pm 5$ | $1.50 \pm 0.04$ |
| | Down-up | $-0.034 \pm 0.006$ | – | $13.9 \pm 0.5$ | $60 \pm 5$ | $1.51 \pm 0.04$ |
| Straight Fig. S3 | Up-down | $-0.007 \pm 0.003$ | $-0.33 \pm 0.10$ | $18.1 \pm 0.7$ | $58 \pm 5$ | $1.56 \pm 0.04$ |
| | Down-up | $-0.011 \pm 0.004$ | $-0.39 \pm 0.11$ | $17.2 \pm 0.7$ | $53 \pm 4$ | $1.54 \pm 0.04$ |

TABLE S1. The fitting parameters for the zigzag and straight wires. The parameter errors originate solely from the standard deviation during data analysis, and the main source of uncertainty is electrical noise.

# 7. DW resistance measurement of other samples

In order to show the reproducibility of the chiral DW resistance, The DW resistance of zigzag wires is measured on another sample with the same stack, i.e., Pt(4 nm)/Co(0.5 nm)/Pt(2 nm). The result shown in Fig. S3 is very similar to Fig. 4(a), and the fitting parameters are also comparable, shown in Table S1 (zigzag #2).

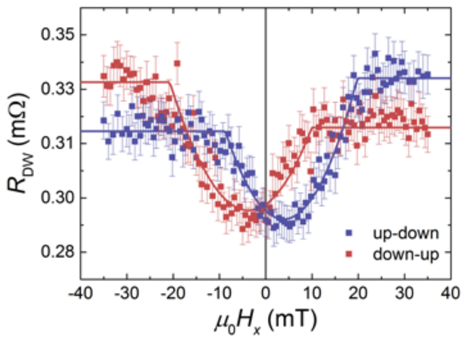


FIG. S4. The measured single DW resistance as a function of in-plane field on a zigzag wire. The blue and red squares represent the magnetic switching with different polarities (up-down and down-up, respectively). The blue and red solid lines are fits to the data based on the theoretical model.

# 8. DW resistance measurement of Pt/Co/AlOx

In order to achieve an artefact-free test of chiral DW resistance, we choose to compare the results on a straight wire and zigzag wire. These two wires are made of the same materials and we made sure all parameters of the two wires are identical, except for the DW chirality, so that we can solely detect the difference caused by the chirality. This is important in our system, since the underlying physics could be rather complicated due to the mixture of many phenomena, e.g., the Rashba effect, the DMI, the AMR, the spin Hall effect, and so forth. As a further confirmation of measuring true chiral DW resistance, our artefact-free data clearly show the anticipated distinct difference between straight and zigzag wires. In addition to the comparison between the straight and zigzag wires, we attempted to further substantiate our test by adopting a structure with tunable DMI/Rashba effect. However, tuning the DMI/Rashba in material/sample is not as simple as it sounds, and the way to determine the magnitude of the DMI/Rashba still remains controversial. On top of that, there are numerous details that complicate the system when comparing different material systems in our delicate zigzag wires. For instance, we have tried to measure the structure suggested to have higher DMI, i.e. Pt/Co/AlOx. However, it turned out that a reliable test was difficult due to a technical problem: the optimal range

of Ga irradiation is too narrow for Pt/Co/AlOx in a zigzag wire and it is thus difficult to achieve controllable DW nucleation. Despite the technical issue in the measurement of Pt/Co/AlOx, for which we decide not to processed further, we believe the clear distinction between zigzag and straight Pt/Co/Pt wire and its accordance with the model can lend a strong support to the exist of chiral DW resistance.


[S1] P. M. Levy and S. Zhang, Phys. Rev. Lett. **79**, 5110 (1997).

[S2] K.-W. Kim, H.-W. Lee, K.-J. Lee, and M. D. Stiles, Phys. Rev. Lett. **111**, 216601 (2013).

[S3] N. L. Schryer and L. R. Walker, J. Appl. Phys. **45**, 5406 (1974).

[S4] A. Kobs, S. Heße, W. Kreuzpaintner, G. Winkler, D. Lott, P. Weinberger, A. Schreyer, and H. P. Oepen, Phys. Rev. Lett. **106**, 217207 (2011).

[S5] A. Thiaville, S. Rohart, É. Jué, V. Cros, and A. Fert, Europhys. Lett. **100**, 57002 (2012).

[S6] The code is available at http//math.nist.gov/oommf.

[S7] H. Nakayama, M. Althammer, Y. T. Chen, K. Uchida, Y. Kajiwara, D. Kikuchi, T. Ohtani, S. Geprägs, M. Opel, S. Takahashi, R. Gross, G. E. W. Bauer, S. T. B. Goennenwein, and E. Saitoh, Phys. Rev. Lett. **110**, 206601 (2013).

[S8] J. Kim, P. Sheng, S. Takahashi, S. Mitani, and M. Hayashi, Phys. Rev. Lett. **116**, 97201 (2016).
